# Supplementary material for: Growable and Interpretable Neural Control with Online Continual Learning for Autonomous Lifelong Locomotion Learning Machines
Source: arXiv:2505.12029 source file (2025-05-17)
Supplement: Supplementary file 1 [file supplementary.tex]

\section{Continual Locomotion Learning Signals}
\refstepcounter{anum}
\label{sec:moresignals}

\begin{figure*}[!h] 
	\centering
	\includegraphics[width=.99\textwidth]{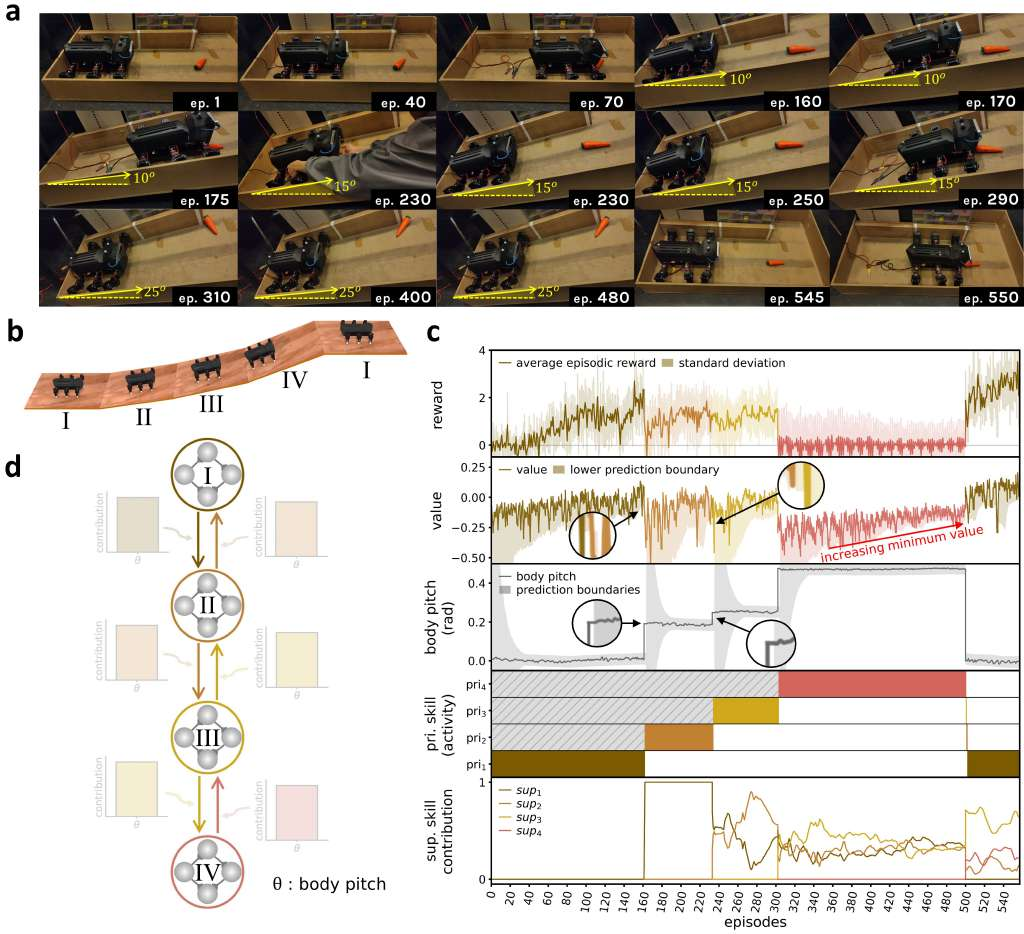}
	\caption{\expmaincaption{on different slopes: (I) 0$^\circ$, (II) 10$^\circ$, (III) 15$^\circ$, and (IV) 25$^\circ$}{odometry pitch}}
	\label{fig:exp_slope}
\end{figure*}

\begin{figure*}[!h] 
	\centering
	\includegraphics[width=0.95\textwidth]{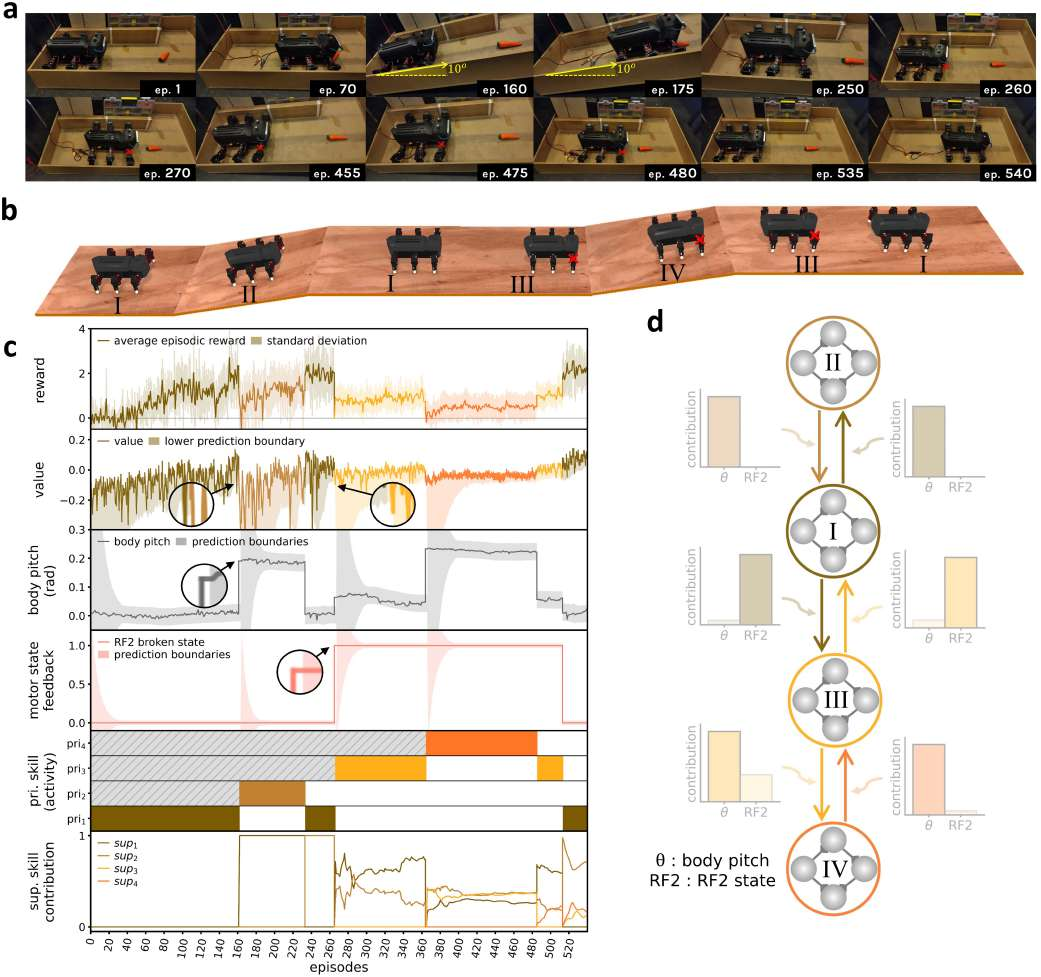}
	\caption{\expmaincaption{on different slopes with possible motor dysfunction: (I) level floor, (II) 10\deg{} slope, (III) level floor with RF2 motor dysfunction, and (IV) 10\deg{} slope with RF2 motor dysfunction}{odometry pitch and RF2 motor dysfunction state}} 
	\label{fig:exp_broken}
\end{figure*}

\begin{figure*}[!h] 
	\centering
	\includegraphics[width=0.99\textwidth]{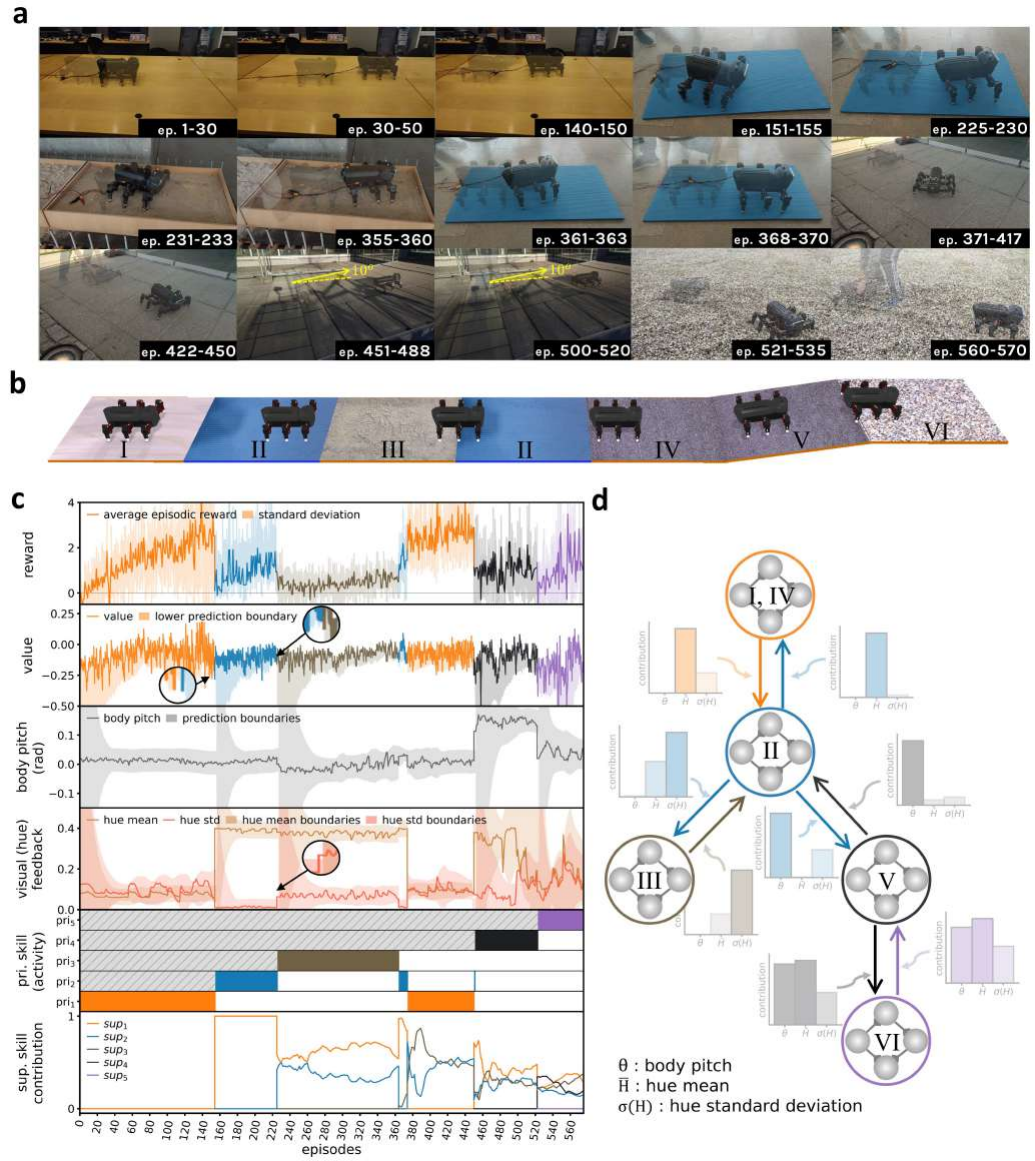}
	\caption{\expmaincaption{on different terrains: (I) \ttable, (II) \bluemat, (III) \sponge, (IV) \rough, (V) \roughslope, and (VI) \gravels}{odometry pitch, average hue pixel, and standard deviation of hue pixel}}
	\label{fig:exp_terrain}
\end{figure*}

\clearpage

\section{Evolution of Foot Trajectories}
\refstepcounter{anum}
\label{sec:foottraj}

\begin{figure*}[htbp]
	\centering
	\includegraphics[width=\linewidth]{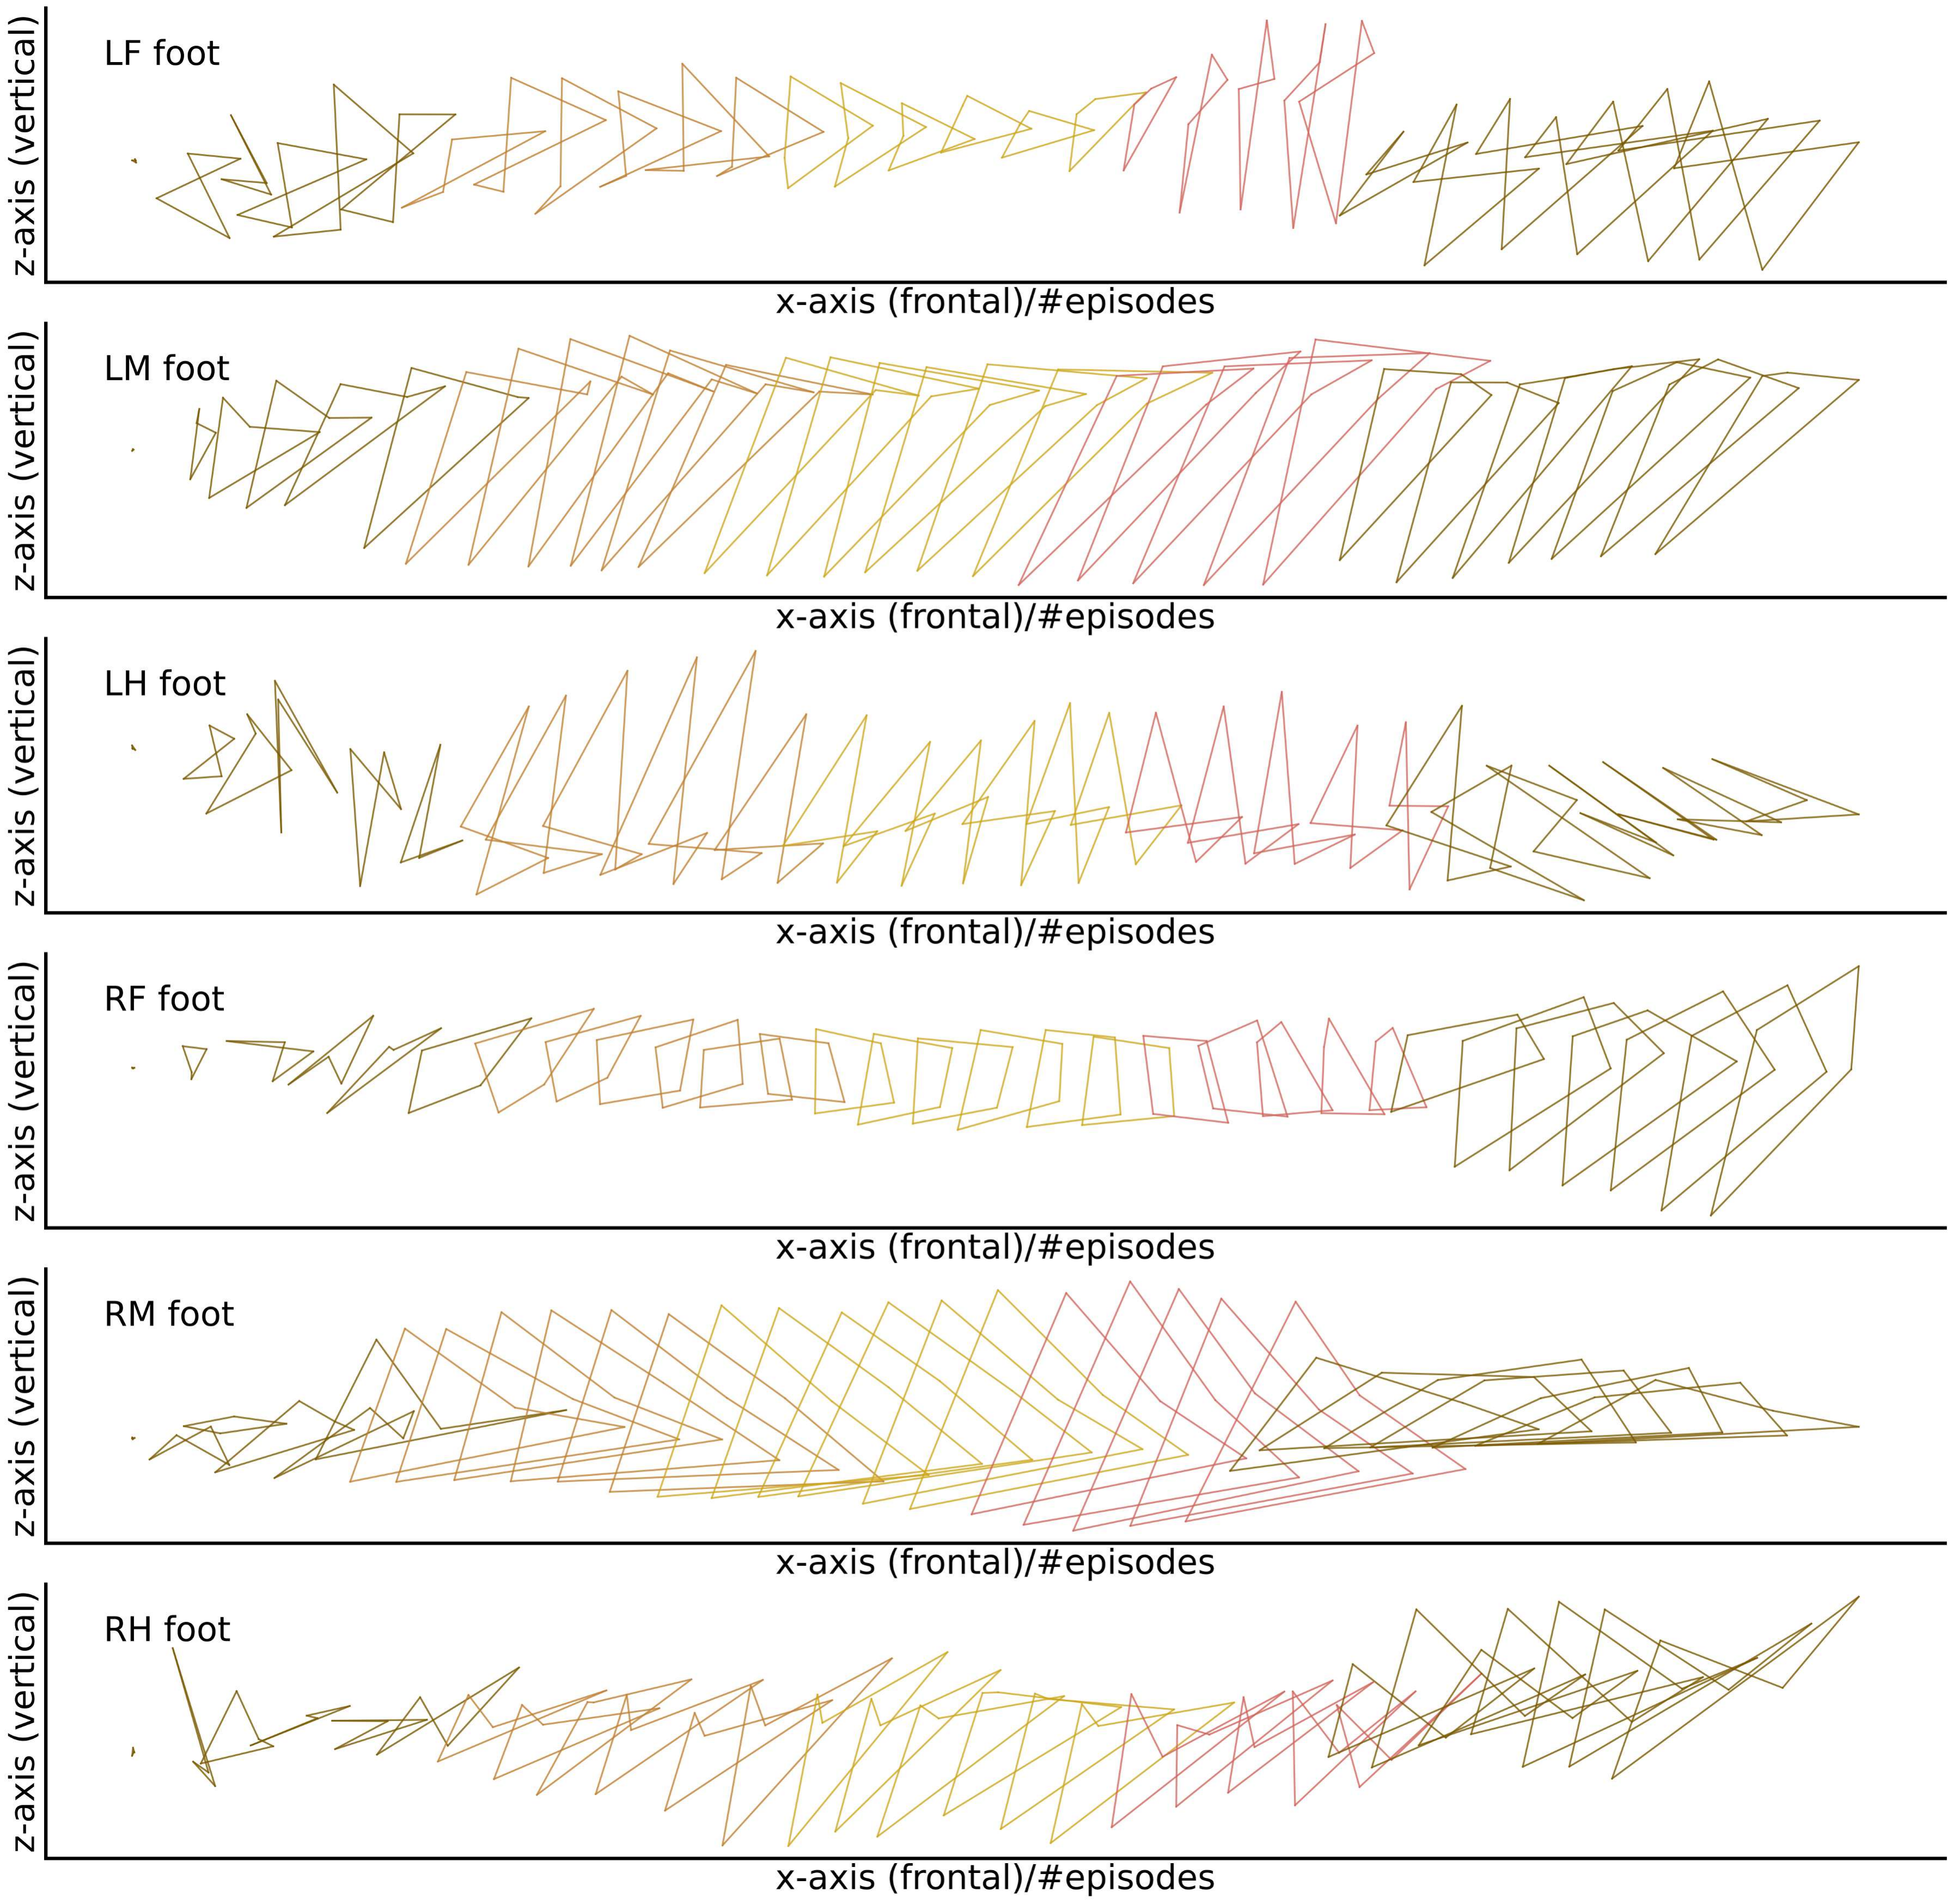}
	\caption{\footcap{different slopes}{second}{\ref{sec:result}}}
	\label{fig:foot_slope}
\end{figure*}

\begin{figure*}[htbp]
	\centering
	\includegraphics[width=\linewidth]{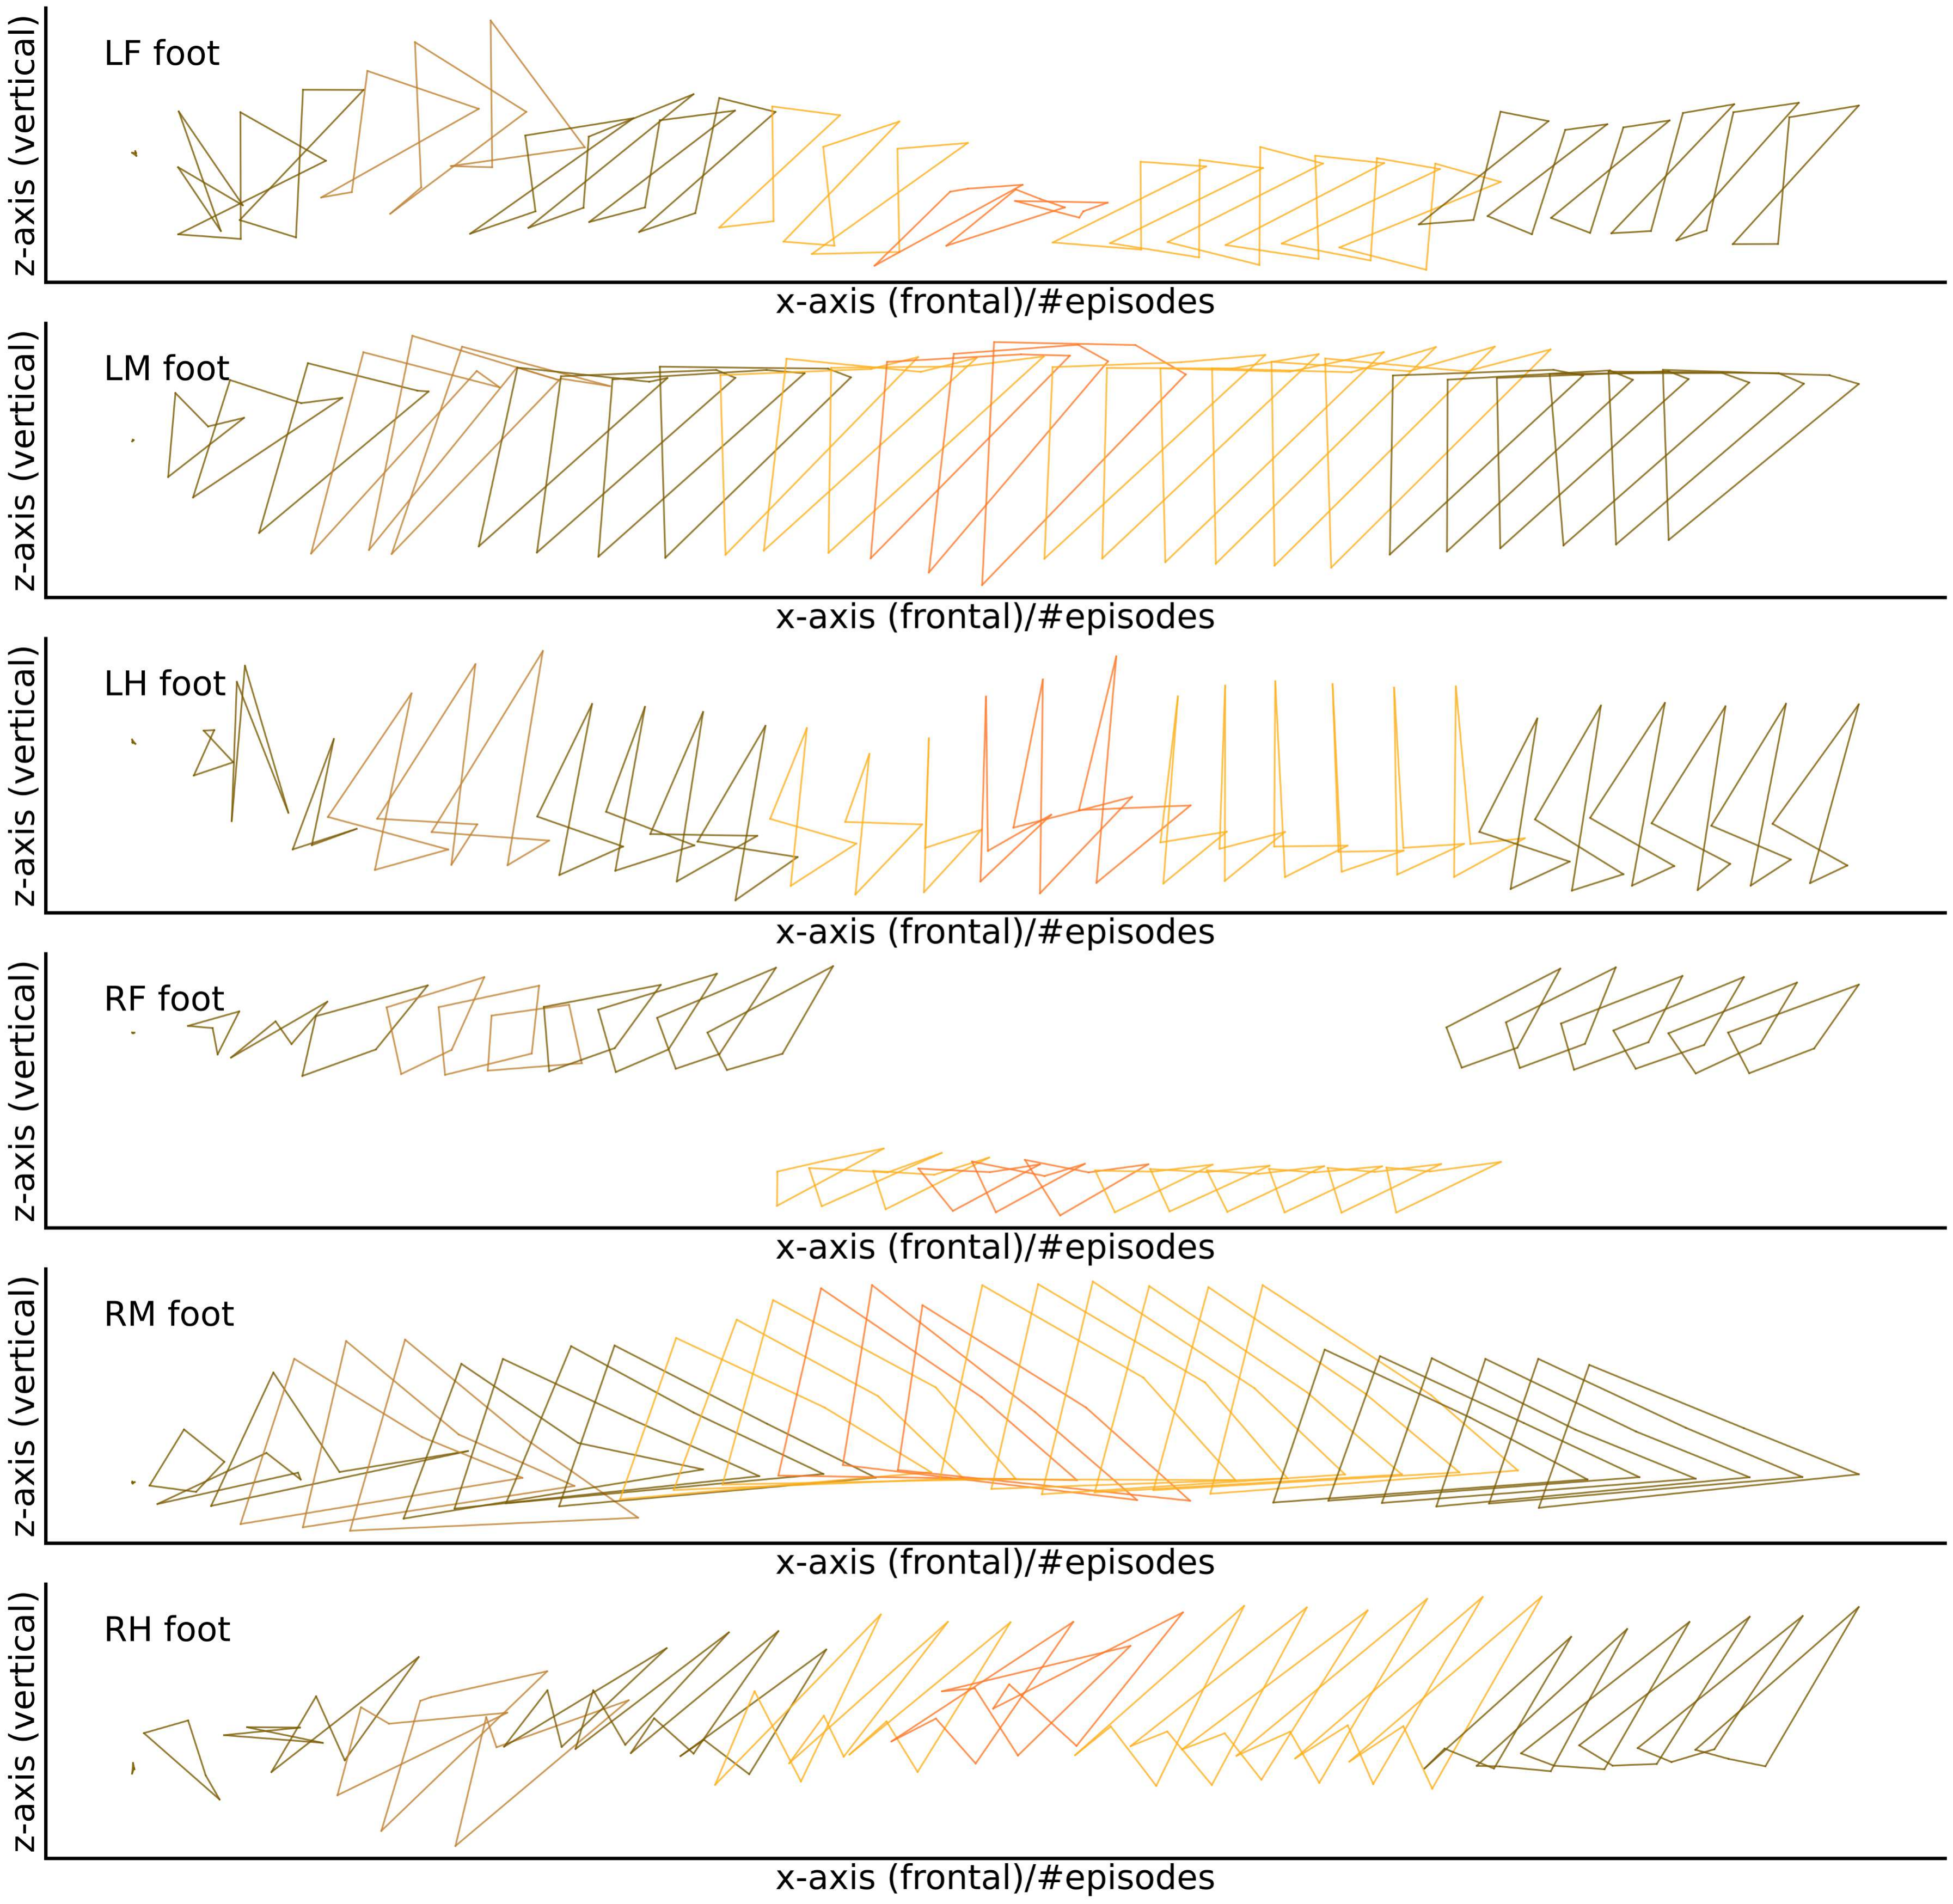}
	\caption{\footcap{different slopes with potential motor dysfunction}{third}{\ref{sec:result}}}
	\label{fig:foot_broken}
\end{figure*}

\begin{figure*}[htbp]
	\centering
	\includegraphics[width=\linewidth]{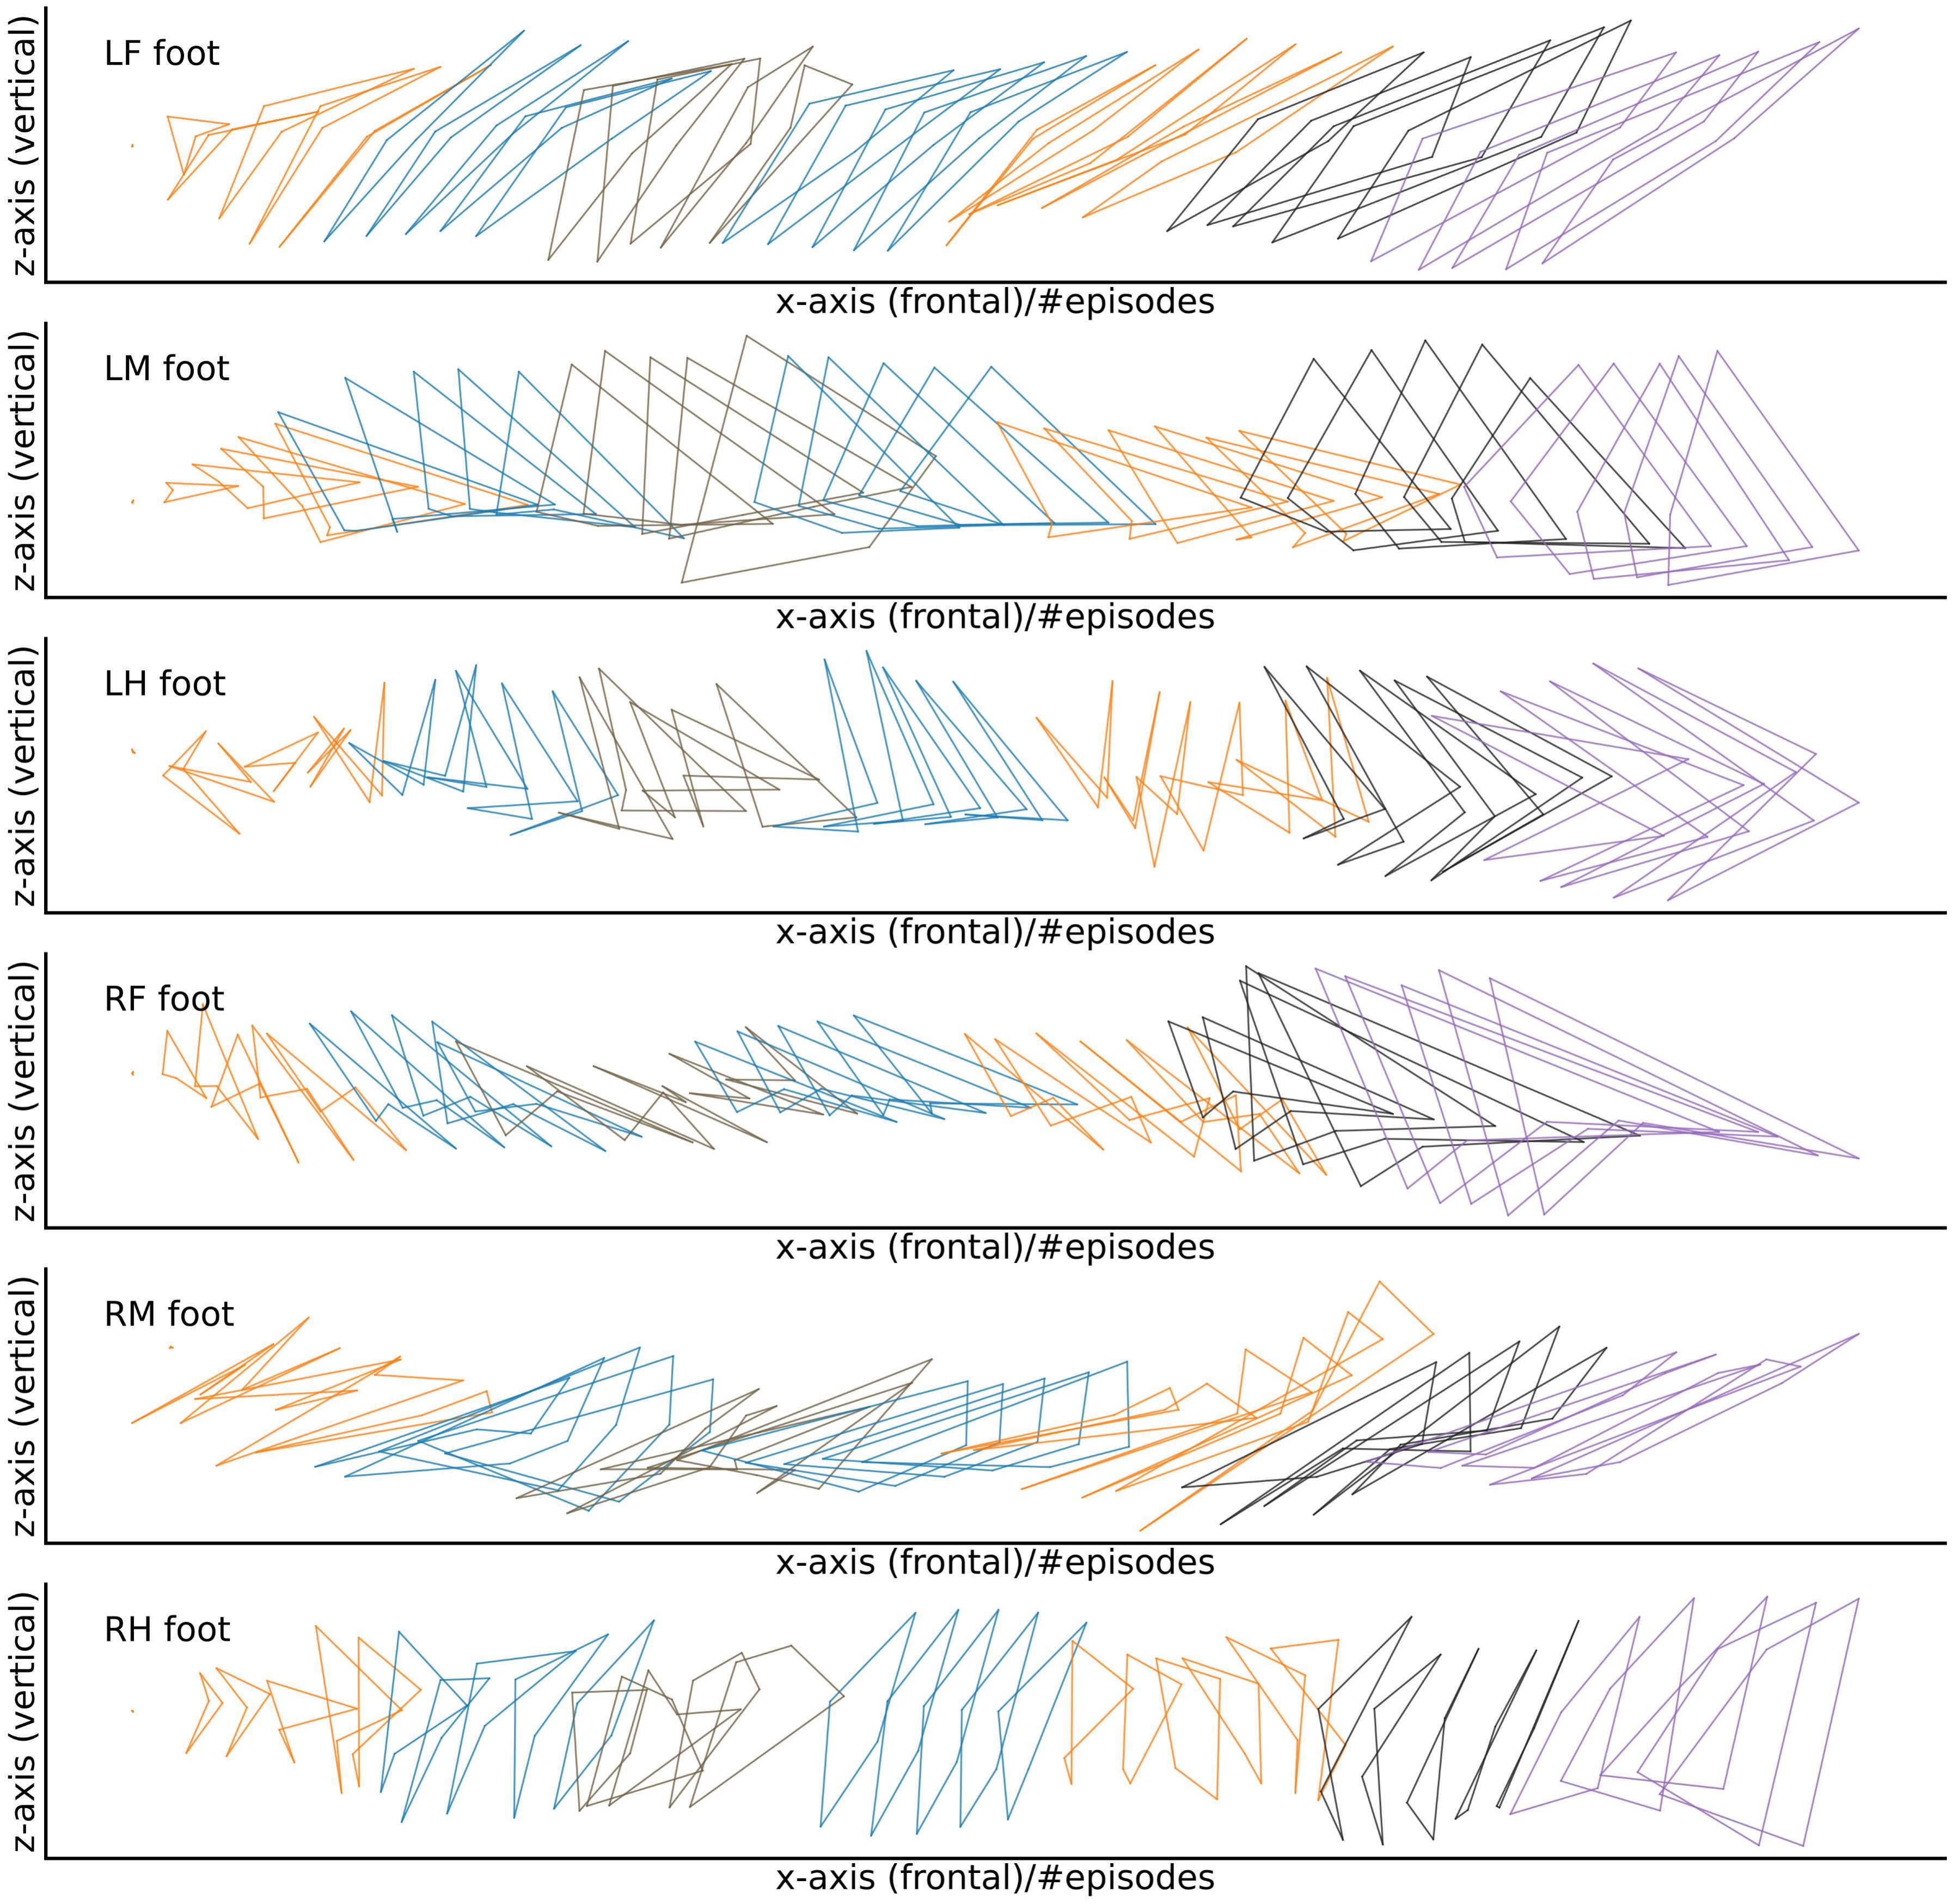}
	\caption{\footcap{different terrains}{fourth}{\ref{sec:result}}}
	\label{fig:foot_terrain}
\end{figure*}

\clearpage

\section{Separation and Incrementation of Knowledge/Skills}
\refstepcounter{anum}
\label{sec:supprimarylearning}

\begin{figure*}[!h] 
	\centering
	\includegraphics[width=0.99\textwidth]{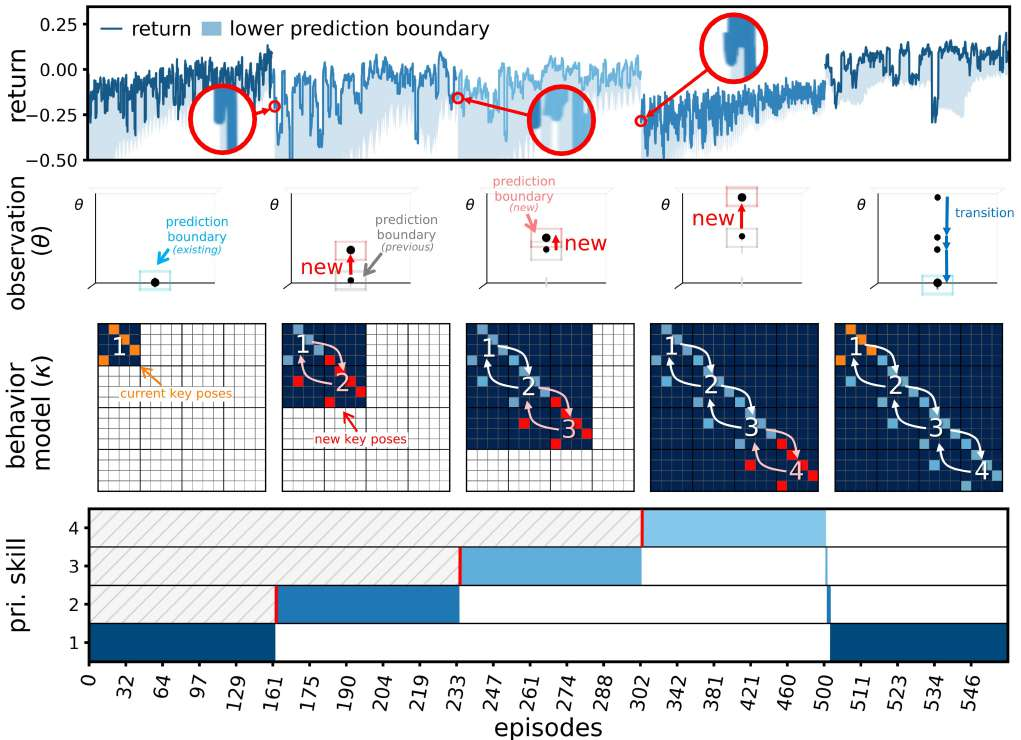}
	\caption{Returns and the lower prediction boundary obtained from energy efficient locomotion learning \firstsequence, trajectory of the sensory feedback in the observation space (body pitch $\theta$) presented along with their prediction boundary and snapshot of the terrains, robot behavior model extracted from and presented along with the transition matrix $\kappa$, i.e., the structure of hidden state connections, where the element at row $i$ and column $j$ ($\kappa_{ij}$) denotes the existence of the transition/positive connection from hidden state $i$ to $j$ and the activation of the primary skills. Note that, throughout this figure, the incrementation of new subnetworks is highlighted in red.}
	\label{fig:supprimarylearning1}
\end{figure*}

\begin{figure*}[!h] 
	\centering
	\includegraphics[width=0.99\textwidth]{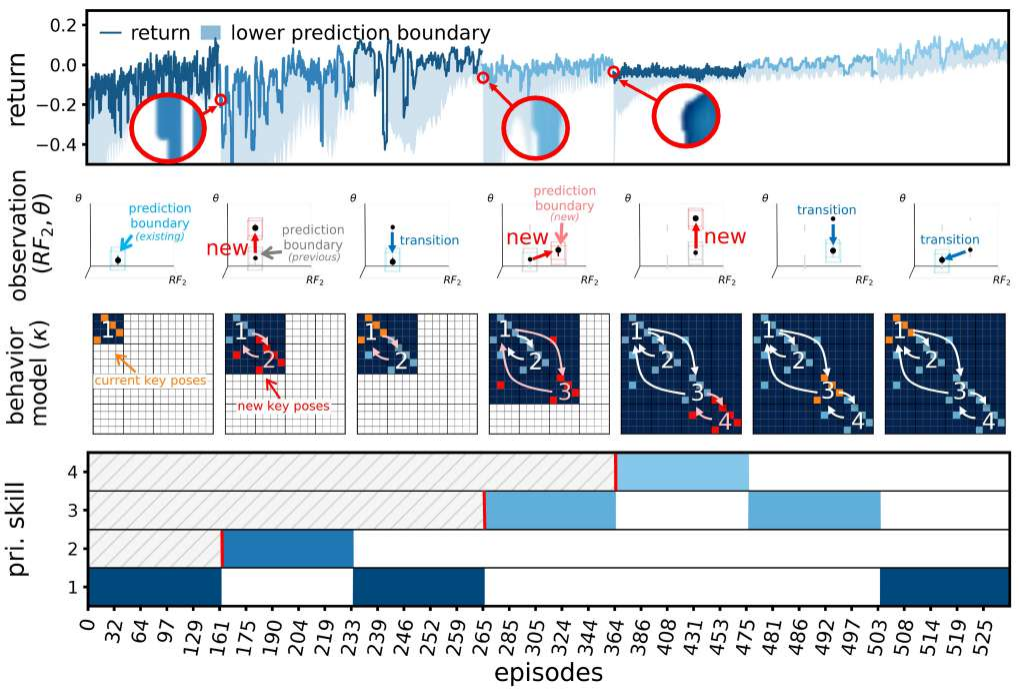}
	\caption{Returns and the lower prediction boundary obtained from energy efficient locomotion learning \secondseqeunce, trajectory of the sensory feedback in the observation space (body pitch $\theta$ and RF2 motor state $RF_2$) presented along with their prediction boundary and snapshot of the terrains, robot behavior model extracted from and presented along with the transition matrix $\kappa$, i.e., the structure of hidden state connections, where the element at row $i$ and column $j$ ($\kappa_{ij}$) denotes the existence of the transition/positive connection from hidden state $i$ to $j$ and the activation of the primary skills. Note that, throughout this figure, the incrementation of new subnetworks is highlighted in red.}
	\label{fig:supprimarylearning2}
\end{figure*}

\clearpage

\section{Quadruped Locomotion Learning}
\refstepcounter{anum}
\label{sec:quadfigures}

In this supplementary section, two types of quadruped locomotion learning are presented to verify the generalization of \frame.


\begin{figure}[!h] 
	\centering
	\includegraphics[width=0.95\textwidth]{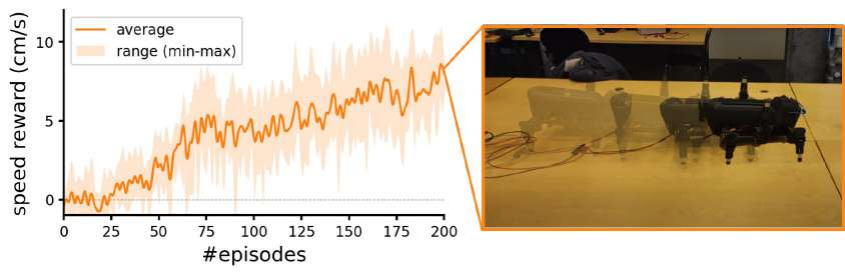}
	\caption{Reward and time-lapse image obtained during locomotion learning with \frame{} on the MORF robot after the amputation of two middle legs (i.e., four-legged MORF version). A video of this experiment is available at \videoquad.}
	\label{fig:quadmorf}
\end{figure}


\begin{figure}[!h] 
	\centering
	\includegraphics[width=0.99\textwidth]{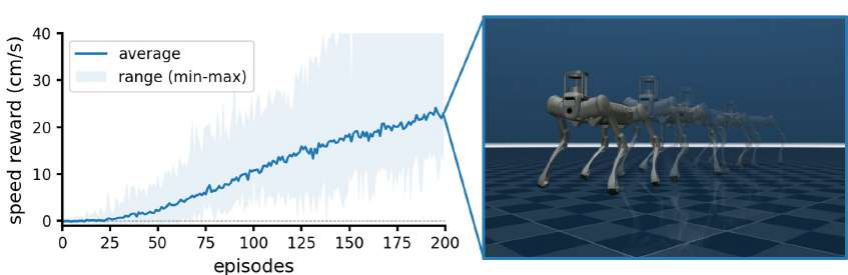}
	\caption{Reward and time-lapse image obtained during locomotion learning with \frame{} on the simulated Unitree B2 quadruped robot. A video of this experiment is available at \videobone.}
	\label{fig:quadbone}
\end{figure}

\clearpage

\section{Bio-inspired Lifelong Learning Feature}
\refstepcounter{anum}
\label{sec:biofeature}

\frame{} exhibits several features of a lifelong learning machine \citep{bio_liftlonglearning}, as summarized in \figlifelong{}. \llfexplain{First}{neurogenesis algorithm}{biological neurogensis and neuromodulation}{s}{increment new subnetwork only when necessary (resource efficiency) and allow online learning (transfer \& adapt) without catastrophic forgetting and task context (task-agnostic learning)} \llfexplain{Second}{\init{} also}{neurogenesis}{}{allows \expsim{} during the increment of new skills (transfer \& adapt)} \llfexplain{Third}{primary learning}{neuromodulation and context gating}{s}{provide also online learning (transfer \& adapt) of relevant skills (overcome forgetting)} \llfexplain{Fourth}{unsupervised hierarchy learning}{context gating, hierarchical system, and sensory integration}{s}{allow autonomous selection/attention of certain important information, such as, certain behaviors/key poses during the learning (task-agnostic and context gated transfer \& adapt), resulting in robustness (noise tolerance)} \llfexplain{Fifth}{supplementary learning}{context gating and hierarchy system}{s}{allow sharing between different highlevel key poses (exploit similarity and transfer \& adapt)} \llfexplain{Sixth}{adaptive exploration}{metaplasticity}{}{allows autonomous exploration rate adaptation (i.e., indirect learning rate adaptation) without any manually provided task-related information (task-agnostic learning)} \llfexplain{Seventh}{short experience replay required}{episodic replay}{}{allows the use of relatively short experience replay for the learning (resource efficiency)}

\begin{figure}[!h]
	\centering
	\includegraphics[width=\linewidth]{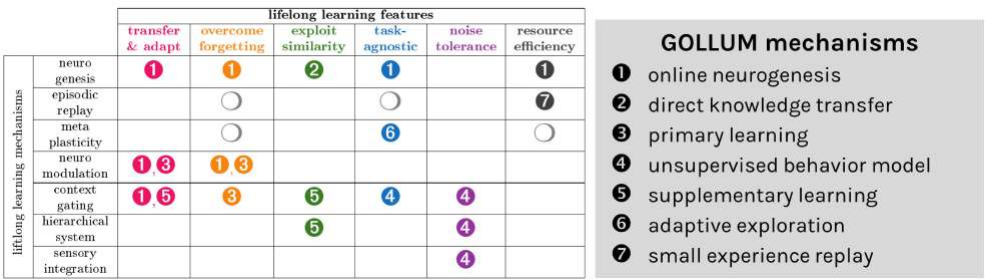}
	\caption{The locomotion learning mechanisms in the \frame{} framework, distributed in terms of lifelong learning features and biological learning mechanisms discussed in \cite{bio_liftlonglearning}, where the reported lifelong learning features and the reported biological mechanisms are organized in columns and rows, respectively. \ding{182}--\ding{188} denote seven learning mechanisms of \frame{}, while \ding{109} denotes the learning mechanisms mentioned in \cite{bio_liftlonglearning} but not included in \frame.}
	\label{fig:lifelongtable}
\end{figure}



\section{Parameter Selection: \ZPGfull{} Layer}
\refstepcounter{anum}
\label{sec:zpgparamanal}

\begin{figure}[!h]
	\centering
	\includegraphics[width=0.8\linewidth]{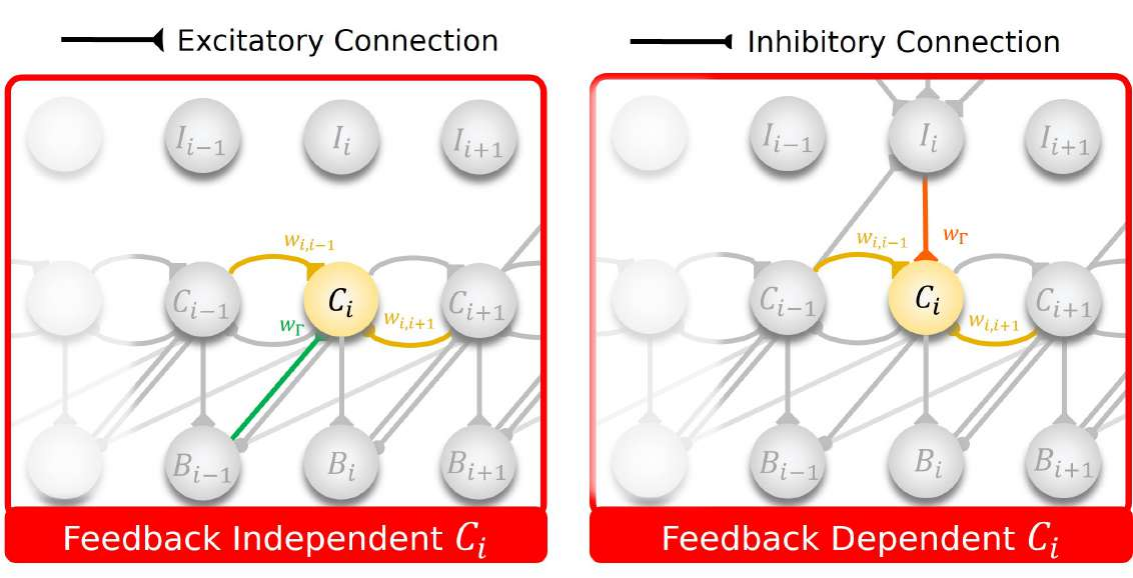}
	\caption{Sub-section of the neural control presented in \figmethod, highlighting $C_k$ and its input signals in case of being (left) sensory feedback-independent and (right) sensory feedback-dependent.}
	\label{fig:zpg_parameterselection}
\end{figure}

In order to select a set of parameters for each \ZPG{} neuron, the entire network is assumed consisting of only 3 \ZPG~neurons, where the middle is used for the selection, as shown in Figure~\ref{fig:zpg_parameterselection}. The activity of neuron $C_k$ can then be simplified as:
\begin{align}
C_i[t+1]  & = \text{sigmoid}(\tilde{C}_i[t+1]) \notag \\
& = \text{sigmoid}(w_{i,i-1} C_{i,i-1}[t] + w_{i,i} C_{i}[t] + w_{i,i+1} C_{i+1}[t] + w_{\Gamma} \Gamma[t] + b_{i}) 
\label{eq:3zpg} 
\end{align} 
\noindent where $C_i[t]$ denotes the activities of the neuron $C_i$ at timestep t, $w_{i,j}$ denotes the connection weight from $C_j$ to $C_i$, $b_i$ denotes the bias of neuron $C_i$, $\Gamma[t]$ denotes the propagation triggering signal at timestep $t$, which is selected as $B_{i-1}[t]$ for feedback independent neurons and $I_i[t]$ for feedback dependent neurons, and $w_{\Gamma}$ denotes the connection weight from those to $C_i$.

Using the aforementioned model, the parameters are chosen analytically according to five boundary conditions with four free parameters representing neuron activation levels: $\epsilon$ represents an inactive activity, $\iota$ represents a fully active activity, $\gamma$ represents an excitation activity ($\epsilon \leq \gamma \leq \iota$), and $\omega$ represents the saturation region of the sigmoid function ($\text{sigmoid}(\omega) \rightarrow 1$).  \\

\noindent \underline{{Propagated Excitation Conditions} }\\
The first boundary condition is that  $C_i$ should be at least an excitation value $\gamma$ ($\tilde{C}_i[t] = \gamma$) when the previous neuron $C_{i-1}$ activates along with $\Gamma$ ( $C_{i-1}[t] = \gamma[t] = \iota$) even if $C_i$ itself and others are inactive ($C_{i}[t] = \epsilon$ and $C_{i+1}[t] = \epsilon$. Eq.~\ref{eq:3zpg} can therefore be rewritten as:
\begin{align}
\gamma & = w_{i,i-1} (\iota) +  w_{i,i} (\epsilon) +  w_{i,i+1} (\epsilon)  + w_{\Gamma} (\iota) + b_{i}.
\label{eq:cond1} 
\end{align} 
However, $C_i$ should not get activated when only $C_{i-1}$ or $\Gamma$ are active. This leads to the second and third boundary conditions as follows:
\begin{align}
-\omega & = w_{i,i-1} (\iota +n\epsilon) +  w_{i,i} (\epsilon) +  w_{i,i+1} (\epsilon)  + w_{\Gamma} (\epsilon) + b_{i},
\label{eq:cond2} \\
-\omega & = w_{i,i-1} (n \epsilon) +  w_{i,i} (\epsilon) +  w_{i,i+1} (\epsilon)  + w_{\Gamma} (\iota) + b_{i}.
\label{eq:cond3} 
\end{align}                                                                                                                               
Note that, to include the activities of other neighbor neurons in case of more than three neighbors, $C_{i-1}[t]$ is added by $n \epsilon$ in Eq.~\ref{eq:cond2}, while $C_{i-1}[t]$ is  $n \epsilon$ in Eq.~\ref{eq:cond3}. \\
\\
\noindent  \underline{{Self-excitation Condition}} \\
The fourth boundary condition is that  $C_i$ should remain active ($\tilde{C}_i[t] = \omega$) when it was active in the previous timestep ($C_i[t] = \iota$) even if others are inactive ($C_{i-1}[t] = C_{i+1}[t] = \Gamma[t] = \epsilon$). Eq.~\ref{eq:3zpg} can then be rewritten as:
\begin{align}
\omega & = w_{i,i-1} (\epsilon) +  w_{i,i} (\iota) +  w_{i,i+1} (\epsilon)  + w_{\Gamma} (\epsilon) + b_{i}.
\label{eq:cond4} 
\end{align} 
\\
\noindent  \underline{{Inhibition Condition}} \\
The fifth boundary condition is that $C_i$ should be inhibited ($\tilde{C}_i[t] = -\omega$) when it the next neuron is active ($C_{i+1}[t] = \iota$) even if others are all active ($C_{i-1}[t] = C_{i}[t] = \Gamma[t] = \iota$) Eq.~\ref{eq:3zpg} can then be rewritten as:
\begin{align}
-\omega & = w_{i,i-1} (\iota) +  w_{i,i} (\iota) +  w_{i,i+1} (\iota)  + w_{\Gamma} (\iota) + b_{i}.
\label{eq:cond5} 
\end{align} 

Eqs.~\ref{eq:cond1}--\ref{eq:cond5} can be rearranged as shown in Eq.~\ref{eq:condmat}, the parameters of which can be solved using the inverse matrix as shown in Eq.~\ref{eq:condmatsolve}. 
\begin{equation}
\newcommand*\w[1]{\makebox[1.5em]{$#1$}}
\begin{bmatrix}
\gamma \\ -\omega \\  -\omega \\ \omega \\ -\omega
\end{bmatrix}
=
\begin{bmatrix}
\w\iota & \w\epsilon & \w\epsilon & \w\iota & \w 1 \\
\iota + n\epsilon & \epsilon & \epsilon & \epsilon & 1 \\
n\epsilon & \epsilon & \epsilon & \iota & 1 \\
\epsilon & \iota & \epsilon & \epsilon & 1 \\
\iota & \iota & \iota & \iota & 1 \\
\end{bmatrix}
\begin{bmatrix}
w_{i,i-1} \\ w_{i,i} \\  w_{i,i+1} \\ w_{\Gamma} \\ b_{i}
\end{bmatrix} ,
\label{eq:condmat}
\end{equation}
\begin{equation}
\newcommand*\w[1]{\makebox[1.5em]{$#1$}}
\begin{bmatrix}
w_{i,i-1} \\ w_{i,i} \\  w_{i,i+1} \\ w_{\Gamma} \\ b_{i}
\end{bmatrix} =
\begin{bmatrix}
\w\iota & \w\epsilon & \w\epsilon & \w\iota & \w1 \\
\iota + n\epsilon & \epsilon & \epsilon & \epsilon & 1 \\
n\epsilon & \epsilon & \epsilon & \iota & 1 \\
\epsilon & \iota & \epsilon & \epsilon & 1 \\
\iota & \iota & \iota & \iota & 1 \\
\end{bmatrix}^{-1}
\begin{bmatrix}
\gamma \\ -\omega \\  -\omega \\ \omega \\ -\omega
\end{bmatrix}, 
\label{eq:condmatsolve}
\end{equation}
\noindent where $\omega$, $\gamma$, $\iota$, and $\epsilon$, are four free parameters, with an additional $n$ represents the maximum number of neighbor neurons, which is set to 10 neurons in this work. $\omega$ is chosen as 6 since $\text{sigmoid}(\omega) \rightarrow 1$ and $\text{sigmoid}(-\omega) \rightarrow 0$, $\gamma$ is then selected as 0.0 which make $\text{sigmoid}(\gamma) = 0.5$, $\iota$ is 0.95, and $\epsilon$ is 0.01. Examples of the results are presented in Figure~\ref{fig:example_zpg_tb}.

\begin{figure}[!h]
	\centering
	\includegraphics[width=0.7\linewidth]{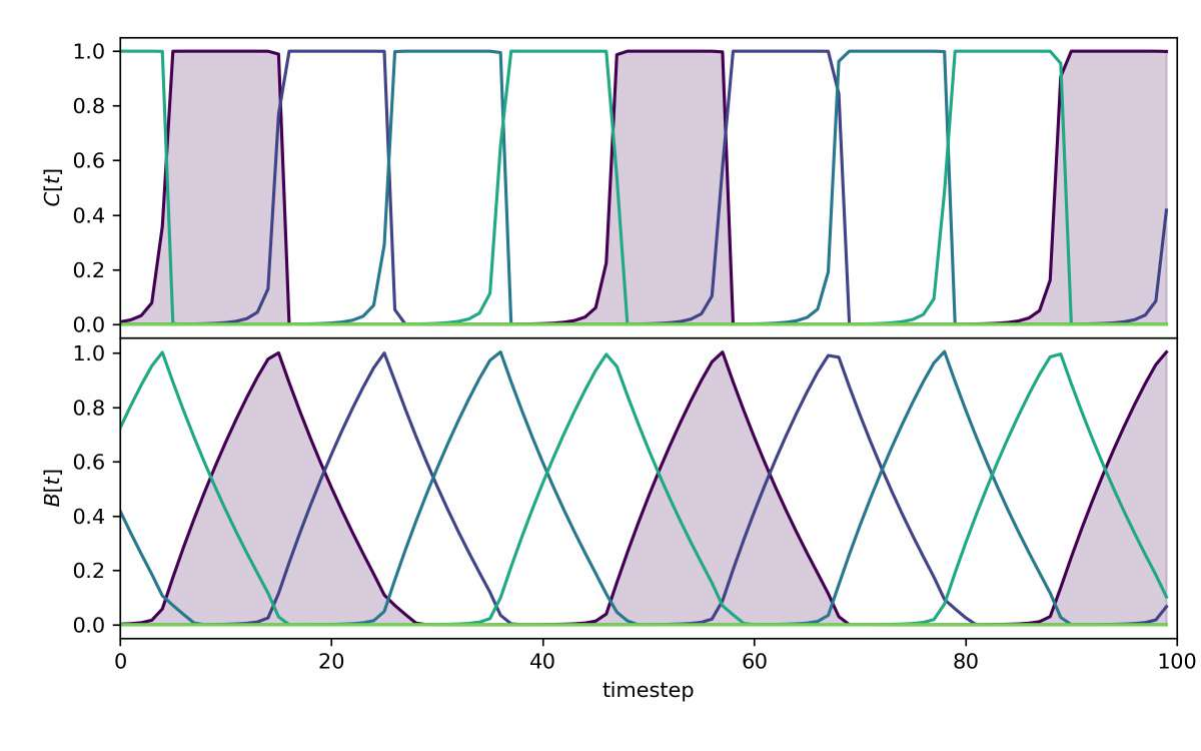}
	\caption{Plot of four \ZPG~activities and four corresponding basis activities.}
	\label{fig:example_zpg_tb}
\end{figure}



\section{Parameter Selection: Basis Layer}
\refstepcounter{anum}
\label{sec:tbparamanal}

The low-pass parameter $w_{B_i,C_{k}}$ and $w_{B_i,B_i}$ in Eq.~\ref{eq:tb} determine the transition speed (i.e., frequency). They together function as low pass filter's parameters: $w_{B_i,C_{k}} = \tau_i$ and $w_{B_i,B_i} = 1- \tau_i$, where $\tau_i$ represents the gain or transition speed parameter corresponding to $C_i$. The higher $\tau_i$ is, the faster the transition speed will be. The relationship between frequency and $\tau_i$ is presented in Figure~\ref{fig:tbn_frequencygraph}.
\begin{figure}[!h]
	\centering
	\includegraphics[width=0.7\linewidth]{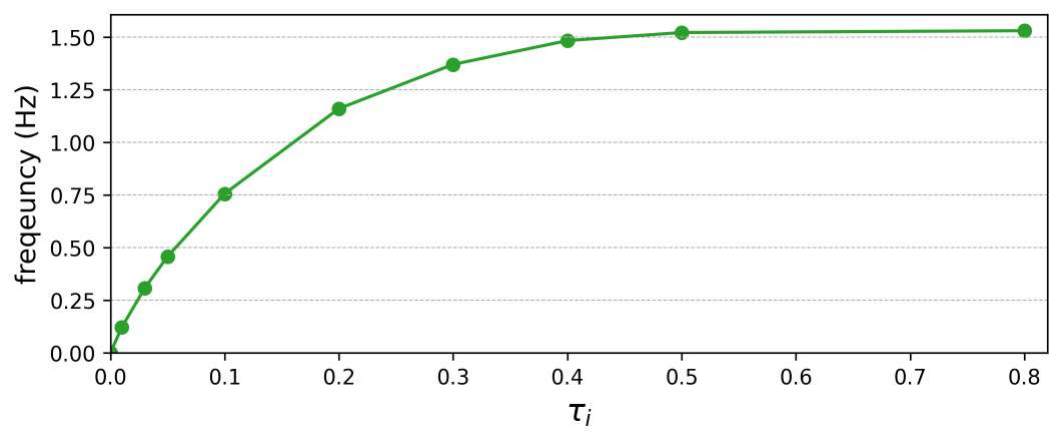}
	\caption{Relationship between $\tau_i$ and the frequency of the basis activities.}
	\label{fig:tbn_frequencygraph}
\end{figure}

To refine the basis shape, the parameters from the next key pose ($w_{B_i,C_{j}}$, where there exists a transition from $C_i$ to $C_j$ ($\kappa_{ij} = 1$)) are empirically set to $-0.5\tau_i$. Correspondingly, those from the second next key pose ($w_{B_i,C_k}$, where there exists a transition from $C_j$ to $C_k$, $\kappa_{jk} = 1$) are empirically selected as $-0.25\tau_i$. These values are selected such that the bases provide less interference between non-neighbors while keeping the mapping outputs smooth, as also illustrated in Figure~\ref{fig:example_zpg_tb}.

With this setup, triangle-shape basis signals are produced, as shown in Figure~\ref{fig:example_zpg_tb}. They are then mapped to smooth interpolation motor outputs. 

\newpage

\begin{figure}
	\centering
	\includegraphics[width=\linewidth]{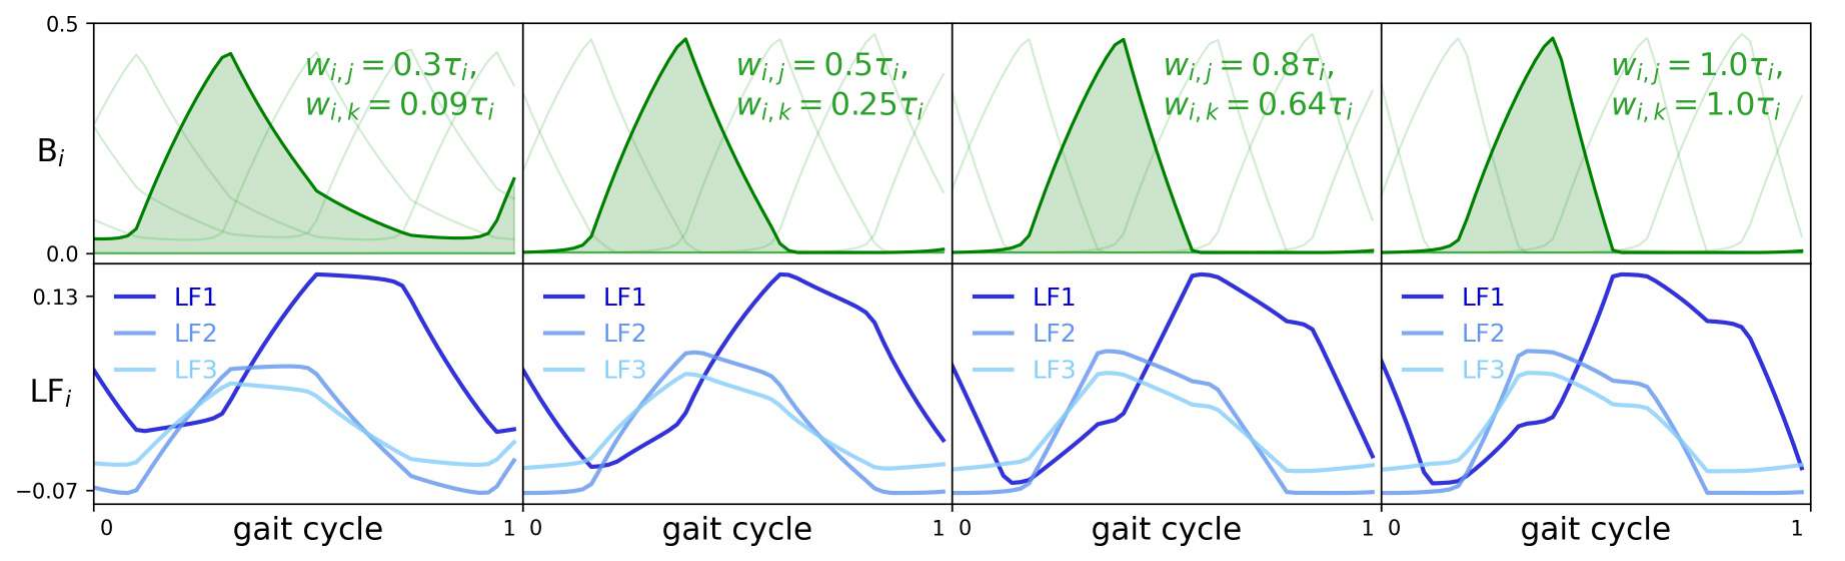}
	\caption{Basis activities and the output motor command obtained from the neural control with ($w_{B_i,C_{j}}$, $w_{B_i,C_{k}} $) = (-0.3$\tau_i$,~-0.09$\tau_i$), (-0.5$\tau_i$,~-0.25$\tau_i$), (-0.8$\tau_i$,~-0.64$\tau_i$), and (-1.0$\tau_i$,~-1.0$\tau_i$). Note that the first pair fails to provide triangle-shape signals, while the last two pairs fails to produce smooth outputs.}
	\label{fig:ipn_decaygain}
\end{figure}

\section{Effect of Value Fitting on the Learning Performance}
\refstepcounter{anum}
\label{sec:valueloss}

\begin{figure}[!h]
	\centering
	\includegraphics[width=0.7\linewidth]{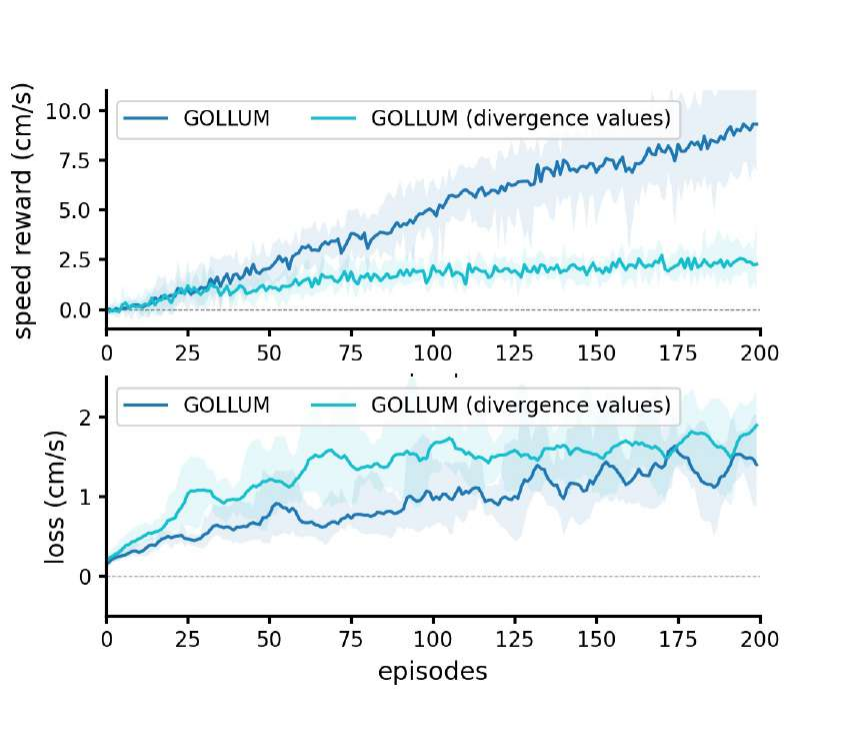}
	\caption{Speed reward obtained from \frame, trained with a value fitting learning rate of 0.2 (blue, selected) and 0.01 (cyan, convergence values). The corresponding value fitting loss is shown below. This presents that using a lower learning rate, aiming to make the value estimation slow and achieve faster learning, leads to erroneous updates (with the root-mean-square error reaching 70\% of the actual reward received). This later leads to poor and unstable results.}
	\label{fig:vloss}
\end{figure}




\section{Scalability Analysis}
\refstepcounter{anum}
\label{sec:scalability}


In our scalability analysis, we recorded the number of parameters and trained parameters as the size of the network increased (i.e., as the number of neurons per layer increased). Figure~\ref{fig:complexity} (left) shows that as \frame{} uses its neural architecture to encode different skills, the number of parameters grows with the number of neurons. However, since most of the fixed parameters in \frame{} are highly structured and sparse, they can be represented using significantly less information. For instance, recent studies \citep{sparsecompress_blockwise,sparsecompress_viterbi} demonstrate that compression algorithms can reduce sparse matrices by 70--85\%. Another approach is parameterizing the network with an $n \times n$ connection matrix ($\kappa$) to represent the network structure and the mapping weight matrices to represent learned mapping parameters. Therefore, the total number of parameters in \frame{} can be compressed significantly. Figure~\ref{fig:complexity} (left) includes an example of 80\% compression, showing that the number of parameters in \frame{} can be even lower than those in 2-hidden layer actor-critic-based (Figure~\ref{fig:complexity} (middle)) and 2-hidden layer actor-twin Q network-based (Figure~\ref{fig:complexity} (right)) neural networks. Moreover, while deep reinforcement learning typically relies on either actor-critic or actor-twin Q network architecture with 256-2048 neurons per layer \citetraining, the equivalent \frame{} network with 4 actions per skill can encode 64-512 distinct skills without catastrophic forgetting.

\begin{figure}[!h]
	\centering
	\includegraphics[width=\linewidth]{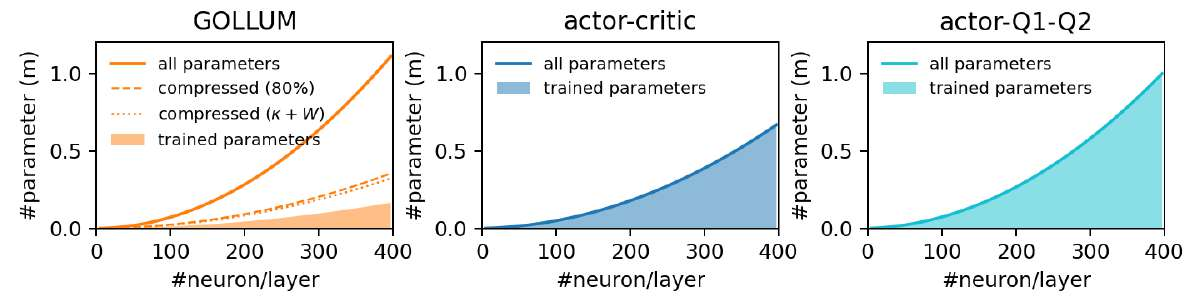}
	\caption{The number of all parameters and trained parameters used in (left) \frame, (middle) 2-hidden layer actor-critic-based, and (right) 2-hidden layer actor-twin Q network-based neural networks, where the number of neurons per layer varies from 0 to 400. Given that most of the fixed parameters of \frame{} are highly structured and sparse, and certain sparse matrix compression algorithms can achieve up to 70--85\% compression ratios \citep{sparsecompress_blockwise,sparsecompress_viterbi}, the total number of parameters in \frame{} can be compressed significantly using an 80\% compression rate (dashed orange line). This can be achieved by compressing both the connection matrix $\kappa$ and learned mapping weights $W$ (dotted orange line).}
	\label{fig:complexity}
\end{figure}

Although it might seem that the network can grow indefinitely, its growth is controlled by the embodied interaction with the environment. As the network grows and the robot learns more skills, there are more options for the robot to choose from, resulting in a less likely that $R[t] < \left( V[t] - V_\delta[t] \right) $) and $| FB_i[t] - O[t] | >  O_{\delta i}[t]$ occur. As the network grows and the robot learns more skills, it attempts to reuse a previously learned skill that has the most similar feedback pattern. The neurogenesis will occur only if the feedback received is different from the expected feedback while the skill receives less reward than expected. An example of this can be seen in Figure~\ref{fig:expprimarylearning} after 374 episodes, where the robot initially tried the locomotion skill on flat terrain and discovered that it could also generalize to rough terrains, so neurogenesis was not activated.

\begin{figure}[!h]
	\centering
	\includegraphics[width=0.7\linewidth]{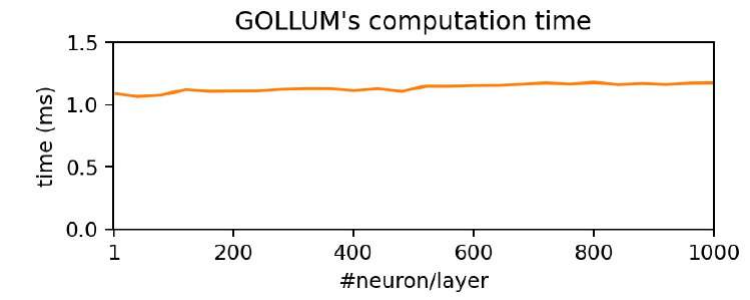}
	\caption{Average computation time per action generation for \frame{} implemented on an Intel Core i7 CPU and NVIDIA GeForce GTX 1050 GPU, with the number of neurons per layer varying from 4 (for 1 behavior/skill) to 1000 (for 250 behaviors/skills).}
	\label{fig:computation}
\end{figure}

Although the network size increases as more behaviors and skills are learned, the average computation time remains below 1.5 ms per action generation, as shown in Figure~\ref{fig:computation}, due to the tensor-based implementation and GPU usage. The computation time shows a slight increase, rising from 1.08 ms to 1.17 ms per action generation. Thus, with 4 to 1000 neurons per layer, or equivalently 1 to 250 behaviors/skills, the control system can operate at over 200 Hz.

\section{Network Parameters}
\refstepcounter{anum}
\label{suc:netparams}
\begin{sidewaystable}[h]
	\centering
	\caption{Summary of the network parameters, their definitions, values, and selection procedure.} \label{tab2}%
	\begin{tabular}{@{}c|c|c | c@{}}
		\toprule
		\bd{Parameter} & \bd{Definition}  & \bd{Value} & \bd{Selection Procedure}\\
		\midrule
		$\kappa$ & connection matrix used to parameterized the structure & changing  & created and modified by the neurogenesis \\
		$w_{I'_i,FB_k}$ & \mc{connection weights from the FB layer to the I' layer\\(feedback contribution/importance)} & changing & trained based on the observation template/prediction \\
		$b_{I'_i}$ & \mc{bias of the I' layer\\(feedback contribution/importance)} & changing & trained based on the observation template/prediction \\
		$w_{I_i,C_k}$ & \mc{connection weights from the C layer to the I layer\\(type of the C neurons)} & 1 or 0 & selected according to on $\kappa$  \\
		$w_{C_i,C_k}$ & \mc{connection weights from with in the C layer\\(\behav)} & 20, 7, -26, or 0 & selected according to on $\kappa$ and Eq.~\ref{eq:condmatsolve}  \\
		$w_{C_i,B_k}$ & \mc{connection weights from the B layer to the C layer\\(type of the C neurons)}  & 7 or 0 & selected according to on $\kappa$ and Eq.~\ref{eq:condmatsolve} \\
		$w_{C_i,I_i}$ & \mc{connection weights from the I layer to the C layer\\(type of the C neurons)}  & 7 or 0 & selected according to on $\kappa$ and Eq.~\ref{eq:condmatsolve} \\
		$b_{C_i}$ & bias of in the C layer & -13 & selected according to Eq.~\ref{eq:condmatsolve}  \\
		$w_{B_i,C_k}$ & \mc{connection weights from the C layer to the B layer\\(transition speed)} & $\tau_i$ & according to $\tau_i$, Figure~\ref{fig:tbn_frequencygraph}, and Figure~\ref{fig:ipn_decaygain}  \\ 
		$w_{B_i,B_i}$ & \mc{recurrent connection weights of the B layer\\(transition speed)} & $1-\tau_i$ & according to $\tau_i$, Figure~\ref{fig:tbn_frequencygraph}, and Figure~\ref{fig:ipn_decaygain}  \\
		$\tau_i$ & transition speed & 0.08 & \makecell{selected empirically based on the desired walking frequency\\according to Figure~\ref{fig:tbn_frequencygraph}} \\
		$w_{PM_i,B_k}$ & \mc{connection weights from the B layer to the PM layer\\(action pattern contribution)} & trained & trained with supplementary learning  \\
		$w_{M_j,PM_k}$ & \mc{connection weights from the PM layer to the output layer\\(motor commands $M_j$)} & trained & trained with primary learning  \\
		$w_{V,B_k}$ & \mc{connection weights from the B layer to the output layer\\(value prediction $V$)} & trained & trained to minimize $\Sigma_t(V[t]-R[t])^2$  \\
		$w_{V_\delta,B_k}$ & \mc{connection weights from the B layer to the output layer\\(maximum value deviation $V_\delta$)} & trained & trained to minimize $\Sigma_t(V_\delta[t]-\max |R[t]-V[t]|)^2$  \\
		$w_{O_i,B_k}$ & \mc{connection weights from the B layer to the output layer\\(observation prediction $O_i$)} & trained & trained to minimize $\Sigma_t(O_i[t]-FB_i[t])^2$  \\
		$w_{O_{\delta i},B_k}$ & \mc{connection weights from the B layer to the output layer\\(maximum observation deviation $O_{\delta i}$)} & trained & trained to minimize $\Sigma_t(O_{\delta i}[t]-\max |O_i[t]-FB_i[t]|)^2$ \\
		$\epsilon_v$ & minimum value of the maximum value deviation & 0.02 & a small positive value \\
		$\epsilon_o$ & minimum value of the maximum value deviation & 0.02 & a small positive value \\
		\bottomrule
	\end{tabular}
	\label{tab:netparam}
\end{sidewaystable}

\clearpage

\section{Training Parameters}
\refstepcounter{anum}
\label{suc:trainingparams}

\begin{table*}[h]
	\centering
	\caption{Summary of the training parameters of \frame, their definitions, and their values. Note that these parameters were selected empirically to obtain fast stable learning ([min,max]).}\label{tab1}%
	\begin{tabular}{@{}c|c|c@{}}
		\toprule
		\bd{Parameter} & \bd{Definition}  & \bd{Value} \\
		\midrule
		$\eta$ & learning rate & 0.5 \\
		$\eta_\sigma$ & learning rate of the exploration rate & 0.05 \\
		$\eta_v$ & learning rate of the value prediction & 0.2 \\
		$\eta_o$ & learning rate of the observation prediction & 0.5 \\
		$\sigma_{\text{min}}$, $\sigma_{\text{max}}$ & minimum and maximum exploration rates & 0.01, 0.05 \\
		$H$ & horizon length & 14 timesteps\\
		$T$ & number of timestep per episode & 30 timesteps\\
		$N_R$ & replay size & 8 episodes\\
		$f$ & controller freqeuncy & 20 Hz \\
		\bottomrule
	\end{tabular}
\label{tab:trainparam}
\end{table*}


\begin{table*}[h]
	\centering
	\caption{Summary of the training parameters of CPGRBF + PIBB \citep{mathias_cpgrbf} and the value/grid search range ([min,max]).}\label{tab2}%
	\begin{tabular}{@{}c|c @{}}
		\toprule
		\bd{Parameter} & \bd{Value(s)} \\
		\midrule
		learning rate & [1e-4,1e-3]  \\
		learning rate of the value prediction & 0.2 \\
		rollout & 8 \\
		number of radial bases & 4 \\
		standard deviation of radial bases & 0.03 \\
		minimum and maximum exploration rates & 0.01, 0.05 \\
		number of timestep per episode & 30 timesteps\\
		controller frequency & 20 Hz \\
		\bottomrule
	\end{tabular}
	\label{tab:trainparam_cpgrbf}
\end{table*}


\begin{table*}[h]
	\centering
	\caption{Summary of the training parameters of DNN + DroQ \citep{droq,walkinthepark} and the value/grid search range ([min,max]).}\label{tab3}%
	\begin{tabular}{@{}c|c @{}}
		\toprule
		\bd{Parameter} & \bd{Value(s)} \\
		\midrule
		learning rate & [3e-4,1e-3]  \\
		learning rate of the value prediction & [3e-4,1e-3] \\
		number of hidden layer & 2 \\
		number of neuron per layer & 256 \\
		activation function & ReLU \\
		buffer memory size & 1e6 \\
		temperature parameter & 5e-3 \\
		entropy coefficient & [0.0,0.2] \\
		number of update per timestep & 20 \\
		layer norm & true \\
		dropout rate & [0.0,0.1] \\
		discounted factor & 0.99 \\
		GAE lambda & 0.95 \\
		exploration standard deviation & [0.01,1.0] \\
		number of timestep per episode & 30 timesteps\\
		controller frequency & 20 Hz \\
		\bottomrule
	\end{tabular}
	\label{tab:trainparam_droq}
\end{table*}

\newpage

\begin{table*}[h]
	\centering
	\caption{Summary of the training parameters of DNN + PPO \citep{ppo,dogrobot_massivelyparallel,dogrobot_teacherstudent} and the value/grid search range ([min,max]).}\label{tab4}%
	\begin{tabular}{@{}c|c @{}}
		\toprule
		\bd{Parameter} & \bd{Value(s)} \\
		\midrule
		learning rate & [3e-4,1e-3]  \\
		learning rate of the value prediction & [1.5e-4,5e-4] \\
		number of hidden layer & 2 \\
		number of neuron per layer & 256 \\
		activation function & Tanh \\
		entropy coefficient & [0.0,0.2] \\
		number of update per episode & 10 \\
		clip ratio & 0.2 \\
		discounted factor & 0.99 \\
		GAE lambda & 0.95 \\
		exploration standard deviation & [0.01,1.0] \\
		number of timestep per episode & 30 timesteps\\
		controller freqeuncy & 20 Hz \\
		\bottomrule
	\end{tabular}
	\label{tab:trainparam_ppo}
\end{table*}


\section{Extension of GOLLUM: Programming Action Sequence by Demonstration}
\refstepcounter{anum}
\label{suc:demo}


To present a possible extension of \frame{}, we keep the interpretable neural control unchanged. However, the learning algorithm is modified as supervised imitation learning, where the reward is replaced by the Dynamic Time Warping (DTW) error, computed from the generated signal and the recorded demonstration sequence. Additionally, the online subnetwork neurogenesis is modified to an offline version, operating with a sliding time window incremental operation.

The processes behind \frame{} are summarized in Algorithm~\ref{alg:programmingbydemo}. First, a demonstration is recorded and preprocessed, as shown in line~\ref{algline:preprocess}. After that, the network transition matrix and the weights are initialized as empty, as shown in line~\ref{algline:initT}. Then, the operation between line~\ref{algline:slidingwindow} and line~\ref{algline:slidenext} is performed under a sliding window operation to incrementally optimize the network connections.

\begin{algorithm}[!h]
	\renewcommand{\algorithmiccomment}[1]{\hfill \textcolor{gray}{{\footnotesize $\#$ #1}}}
	\caption{\frame{} (a variant of \frame{})}\label{alg:programmingbydemo}
	\begin{algorithmic}[1]
		\Require demonstration $\mathcal{D}$, window size $\Delta t$, maximum learning iteration $I_{\text{max}}$, initial neural number $N_{0}$, acceptable error $e^*$
		\Ensure network ($T_{n \times n}$ and $W_{\text{MN,ON}}$)
		
		\State preprocess the demonstration $\mathcal{D}$ \label{algline:preprocess}
		\State initialize empty transition matrix $T$, and zero weight $W_{\text{MN,ON}}$ \label{algline:initT}
		
		\State $t \gets 0$  \label{algline:inittime}
		\While{$t+\Delta t < \mathcal{D}$.size } \Comment{perform sliding window operation} \label{algline:slidingwindow}
		
		\State generates motor command $O[t:t+\Delta t]$ with $\bar{W}_{\text{MN, ON}}$ \label{algline:oldfit}
		\State $e \gets \text{DTW}_e\left( \mathcal{D}[t:t+\Delta t], O[t:t+\Delta t] \right) $ \label{algline:olderror}
		
		\If {$e \geq e^*$} \label{algline:oldcompare}
		
		\State $\bar{T} \gets$ network with $N_{0}$ neurons arrange in one loop transition \label{algline:initTbar}
		\State fit $\bar{W}_{\text{MN, ON}}$ to $\mathcal{D}[t:t+\Delta t]$ \label{algline:fit}
		\For{$i \in [0,I_{\text{max}}]$} \Comment{optimized network structure} \label{algline:optloop}
		\State $T' \gets$ randomly perturb $\bar{T} $ \label{algline:purturb}
		\State generates motor command $O[t:t+\Delta t]$ with $\bar{W}_{\text{MN, ON}}$ \label{algline:outputcal}
		\State $e \gets \text{DTW}_e\left( \mathcal{D}[t:t+\Delta t], O[t:t+\Delta t] \right) $ \label{algline:errorcal}
		\If {$e \leq e^*$} \label{algline:checkerror}
		\State $A \gets (e^*-e)\text{clip}(\bar{T}\text{.size}-T'\text{.size},0,1)$ \label{algline:advantagecal}
		\State $\bar{T} \gets \bar{T} + |Rel_{T'}| (T'-\bar{T}) A $ \label{algline:learnT}
		\EndIf
		\EndFor
		\State append $T$ with the first half of $\bar{T}$  \label{algline:updateT}
		\State append $W_{\text{MN, ON}}$ with the corresponding $\bar{W}_{\text{MN, ON}}$ \label{algline:updateW}
		\State $t \gets t + 0.5\Delta t$ \label{algline:slidenext}
		\EndIf
		\EndWhile
		
	\end{algorithmic}
\end{algorithm}


In the optimization process, a temporary network is created in the first step according to the transition matrix $\bar{T}$, initialized in line~\ref{algline:initTbar}, and the mapping weights $\bar{W}_{\text{MN, ON}}$, which are fit using the demonstration as the target in line~\ref{algline:fit}. Subsequently, the parameter $\bar{T}$ is perturbed, as shown in line~\ref{algline:purturb}, and the corresponding motor commands are generated, as shown in line~\ref{algline:outputcal}. In line~\ref{algline:errorcal}, Dynamic Time Warping (DTW) is performed to align the demonstration with the produced motor commands, and the error is then computed. Lines~\ref{algline:errorcal}--\ref{algline:learnT} compare the fitting error, compute the advantage estimate, and update the temporary transition matrix accordingly. Note that, in this case, the relevance terms are estimated by the activation of the corresponding \ZPG~neuron to simplify the process. All these steps iterate for $I_{\text{max}}$ iterations to prune the network while maintaining an acceptable fitting error (within the acceptance error $e^*$).

After the optimization loop ends, only the first halves of the parameters are appended to the network parameters, as shown in line~\ref{algline:updateT} and line~\ref{algline:updateW}. Finally, the sliding window progresses forward, as shown in line~\ref{algline:slidenext}, and the optimization reiterates. Note that the optimization is skipped if the network with parameters $T$ and $W_{\text{MN, ON}}$ can reproduce the motor commands well, achieving a low acceptable fitting error. The results are illustrated in \videodemo{} (robotic arm manipulation) and \videodemomorf{} (legged robot).
